# Supplementary material for: Manipulating Anomalous Hall Antiferromagnets with Magnetic Fields
Source: arXiv:1802.03044 ancillary file (2019-05-14)
Supplement: Supplementary file 1 [file morb-afm-supp-rev.pdf]

# Supplementary Materials for "Manipulating Anomalous Hall Antiferromagnets with Magnetic Fields"

Hua Chen,[1,2] Tzu-Cheng Wang,[3] Di Xiao,[4] Guang-Yu Guo,[3,5] Qian Niu,[6] and Allan H. MacDonald[6]

[1]*Department of Physics, Colorado State University, Fort Collins, CO 80523, USA*
[2]*School of Advanced Materials Discovery, Colorado State University, Fort Collins, CO 80523, USA*
[3]*Department of Physics and Center for Theoretical Physics, National Taiwan University, Taipei 10617, Taiwan*
[4]*Department of Physics, Carnegie Mellon University, Pittsburgh, PA 15213, USA*
[5]*Physics Division, National Center for Theoretical Sciences, Hsinchu 30013, Taiwan*
[6]*Department of Physics, the University of Texas at Austin, Austin, TX 78712, USA*

## DETAILS OF DENSITY FUNCTIONAL THEORY CALCULATIONS

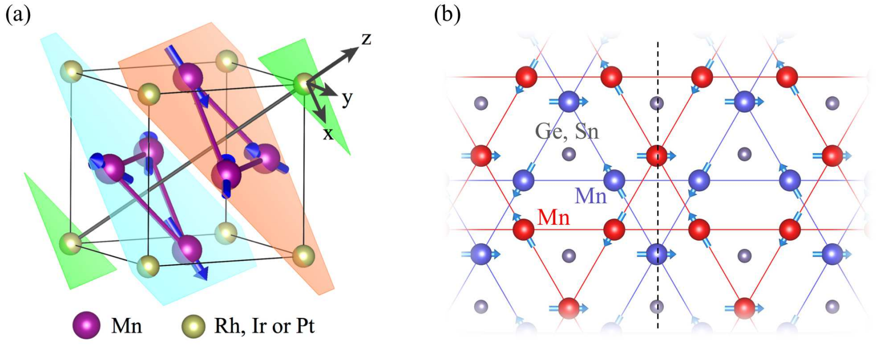


FIG. 1: (a) Crystalline and antiferromagnetic structures of $Mn_3X$ (X = Ir, Pt, Rh); (b) Crystalline and antiferromagnetic structures of $Mn_3X$ (X = Sn, Ge).

$Mn_3X$ (X = Ir, Pt, Rh) form the cubic $L1_2$-type structure with space group $Pm\bar{3}m$ (see [1, 2] and references therein). Here Mn atoms sit at the centers of the faces of the cubic unit cell while X atoms take up the corner positions. In this paper we use the experimental lattices of 3.81, 3.83 and 3.78 Å for $Mn_3Ir$, $Mn_3Pt$ and $Mn_3Rh$ (see [2] and references therein), respectively. We consider the low-energy T1 noncollinear antiferromagnetic structure [2], as illustrated in Fig. S1 (a). In this T1 magnetic structure, the Mn magnetic moments lie in the (111) plane and point to the center of the triangle, forming three nearest-neighboring Mn sublattices, which can be viewed as two-dimensional kagome lattices. In this structure, only the (111) component of the anomalous Hall conductivity tensor ($\sigma^{111}$) and magnetic moments can be nonzero because of the symmetry constraint. In contrast, $Mn_3X$ (X = Sn, Ge) crystalize in the layered hexagonal $DO_{19}$ structure with space group $P6_3/mmc$ [Fig. S1(b)]. The primitive unit cell contains two layers of Mn triangles stacked along the $c$ axis, and in each layer the three Mn atoms form a kagaome lattice with the X atom located at the center of each hexagon. Here we adopt the experimental lattice constants of $a = 5.66$ Å and $c = 4.31$ Å, and $a = 5.66$ Å and $c = 4.31$ Å for $Mn_3Sn$ and $Mn_3Ge$, respectively (see [3] and references therein). Again, here we consider only the low-energy A-type noncollinear antiferromagnetic structure [Fig. S1(b)] [3]. In this magnetic structure, only the $x$ component of the anomalous Hall conductivity tensor ($\sigma_{yz}$) and magnetic moments can be nonzero due to the symmetry.

The electronic and magnetic properties of $Mn_3X$ (X = Ir, Pt, Rh, Sn, Ge) are calculated based on the density functional theory (DFT) with the generalized gradient approximation (GGA) [4]. The pseudopotential plane wave electronic structure method, as implemented in the open-source code Quantum Espresso[5], is used. The fully relativistic norm-conserving pseudopotentials for Mn, Ir, Pt, Rh, Sn and Ge are generated by using the pseudopotential generation code ONCVPSP[6]. The valence electron configurations considered are Mn: $3s3p3d^54s^2$, Ir: $5s5p5d^76s^2$, Pt: $5s5p5d^96s^1$, Rh: $4s4p4d^85s^1$, Sn: $4d^{10}5s^25p^2$ and Ge: $4d^{10}5s^25p^2$. A large energy cutoff for the plane wave (charge density) expansion of 100 Ry (400 Ry) is adopted. In the self-consistant electronic structure calculations, a fine Monkhorst-Pack $k$-point mesh of $15 \times 15 \times 15$ is used for the Brillouin zone (BZ) integration and the total energy

convergence criterion is $10^{-8}$ Ry. The calculated relativistic band structures of $Mn_3Rh$ and $Mn_3Ge$ are displayed, respectively, in Fig. S2(a) and Fig. S3(a), as examples. The band structure of $Mn_3Ge$ shown in Fig. S3(a) is in good agreement with that reported in [3].

The anomalous Hall conductivity (AHC) and orbital magnetic moment are calculated based on the Berry-phase formalism[7]. Within this formalism, the AHC is evaluated as a BZ integration of the Berry curvature for all the occupied bands[7]

$$\sigma = -\frac{e^2}{\hbar}\sum_n \int_{BZ} \frac{d\mathbf{k}}{(2\pi)^3}\mathbf{\Omega}_n(\mathbf{k})f(\epsilon_{n\mathbf{k}}) \tag{1}$$

where $\mathbf{\Omega_n}(\mathbf{k})$ is the Berry curvature for the $n$th band at $\mathbf{k}$ and $f(\epsilon_{n\mathbf{k}})$ is the Fermi-Dirac distribution. Similarly, the orbital magnetization is given as

$$\begin{aligned} \mathbf{M}_{orb} &= \sum_{n\mathbf{k}} \left[\mathbf{m}_n(\mathbf{k})f(\epsilon_{n\mathbf{k}}) + \frac{e}{\hbar}\mathbf{\Omega}_n(\mathbf{k})(\mu - \epsilon_{n\mathbf{k}})f(\epsilon_{n\mathbf{k}})\right] \\ &= \mathbf{M}^1_{orb} + \mathbf{M}^2_{orb}. \end{aligned} \tag{2}$$

where $\mathbf{m}_n(\mathbf{k})$ is the orbital magnetic moment for the $n$th band at $\mathbf{k}$, and $\mu$ is the chemical potential.

To obtain accurate AHC and orbital magnetization, a very dense $k$-point mesh would be needed. Therefore, here we use the very efficient Wannier-interpolation method[8, 9] to calculate these quantities. The maximally-localized Wannier functions [10] are constructed using the wannier90 code [11]. We first calculated the *ab initio* wavefunction by a non-self-consistent calculation using the $8 \times 8 \times 8$ $k$-point mesh. We then projected the wavefunction onto the atomic orbitals $sp^3d^2, d_{xy}, d_{yz}$ and $d_{xz}$ for Mn, Rh, Ir, Pt, Ge and Sn. The 'frozen window' maximum for disentanglement procedure is at least 4 eV above Fermi level. The spread convergence threshold for both disentanglement and wannierization is $10^{-8}$ Å$^2$. The band structures calculated using these obtained Wannier functions are in very good agreement with the corresponding *ab initio* band structures, as demonstrated in Fig. S2(a) for $Mn_3Rh$ and Fig. S3(a) for $Mn_3Ge$. Finally, we used the very dense $101 \times 101 \times 101$ $k$-point mesh to calculate the orbital magnetization and the $151 \times 151 \times 151$ mesh for the AHC calculation. The variation is within 1 % when a denser $k$-point mesh is used. The calculated AHCs for $Mn_3Sn$ (132 S/cm) and $Mn_3Ge$ (276 S/cm) agree well with that [$Mn_3Sn$ (132 S/cm) and $Mn_3Ge$ (298 S/cm)] reported previously[3]. The calculated spin and orbital magnetic moments are listed in Table I in the main text.

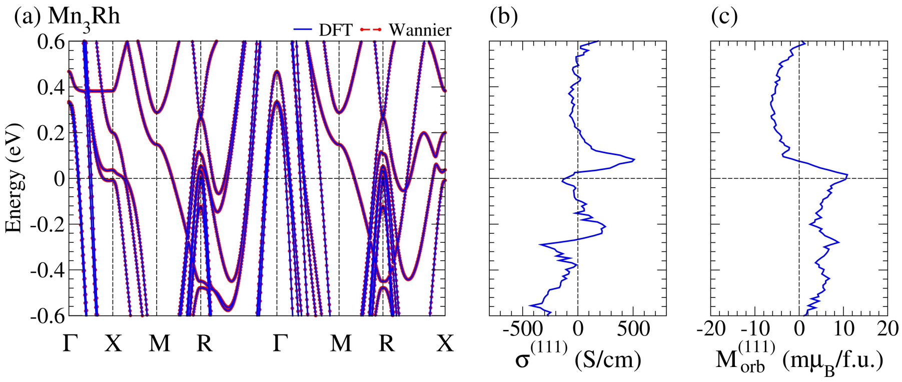


FIG. 2: $Mn_3Rh$. (a) Relativistic band structure from the GGA calculation (blue solid lines) and the Wannier interpolation (red dashed lines). (b) Anomalous Hall conductivity ($\sigma^{111}$) and (c) orbital magnetic moment ($M^{111}_{orb}$) as a function of energy.

## POWER LAW DEPENDENCE OF SPIN CANTING AND ORBITAL MAGNETIZATION ON SPIN-ORBIT COUPLING

Both the spin canting and the orbital magnetization are results of the spin-orbit coupling. In the weakly itinerant limit we can approximate the spin-orbit coupling by its atomic form

$$H_{so} = \lambda_{so}\mathbf{l}\cdot\mathbf{s}. \tag{3}$$

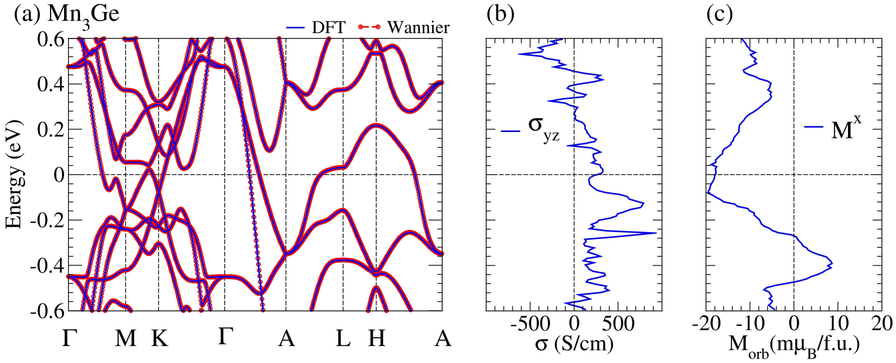


FIG. 3: $Mn_3Ge$. (a) Relativistic band structure from the GGA calculation (blue solid lines) and the Wannier interpolation (red dashed lines). (b) Anomalous Hall conductivity ($\sigma^{111}$) and (c) orbital magnetic moment ($M_{orb}^{111}$) as a function of energy.

We consider the case in which the spin-orbit coupling can be treated as a perturbation over the ground state obtained from the local spin-density approximation. In this case the spin operator in $H_{so}$ can be replaced by the ground state local spin density $s\hat{\Omega}$ where both the amplitude $s$ and the direction $\hat{\Omega}$ are position dependent. The spin-orbit coupling then becomes

$$H_{so} \approx -\left(-\frac{\mu_B}{\hbar}\mathbf{l}\right)\cdot\left(\frac{\hbar\lambda_{so}}{\mu_B}s\hat{\Omega}\right) \equiv -\mathbf{M}_{orb}\cdot\mathbf{H}. \tag{4}$$

The local spin density thus acts as an orbital magnetic field. The orbital magnetization is then obtained as the orbital-orbital susceptibility $\overleftrightarrow{\chi}_o$, calculated in the absence of $H_{so}$, times this orbital magnetic field:

$$\langle\mathbf{M}_{orb}\rangle = \overleftrightarrow{\chi}_o\cdot\mathbf{H} \propto \lambda_{so}. \tag{5}$$

In the case of noncollinear antiferromagnets the local orbital field $\mathbf{H}$ is usually not along the direction of the total orbital magnetization. This can be understood as a result of the anisotropy in the local $\overleftrightarrow{\chi}_o$ that is allowed by symmetry. For example, the structure of $Mn_3Ir$ has a four-fold rotational symmetry around an axis (taken as $\hat{z}$) through a Mn atom and perpendicular to the square formed by its four nearest neighboring Ir atoms (taken as the $xy$ plane). There are also two mirror planes perpendicular to $\hat{x}$ and $\hat{y}$, respectively. These symmetry operations will eliminate all off-diagonal elements of $\overleftrightarrow{\chi}_o$ and make $\chi_o^{xx} = \chi_o^{yy}$, but leave the ratio between $\chi_o^{zz}$ and $\chi_o^{xx}$ unfixed. Thus although $\hat{n}_{111}\cdot\mathbf{H} = 0$, with $\mathbf{H}$ indicated by the arrow on site 3 in Fig. 2 (a) in the main text, $\hat{n}_{111}\cdot\overleftrightarrow{\chi}_o\cdot\mathbf{H} \neq 0$. It is also easy to see that the contributions from the other two sites in the unit cell are the same.

In the main text we have shown that by one can use a similar argument to arrive at the conclusion that the canting-induced total spin magnetization is at least of the 2nd order in $\lambda_{so}$, since $\overleftrightarrow{\chi}_{so}$ must vanish when $\lambda_{so} = 0$. Here we show that this 2nd order dependence can also be obtained by considering magnetocrystalline anisotropy.

Following Bruno[12], we can write the spin-orbit coupling term into an anisotropy energy

$$E_{so} = -\frac{1}{2}\mathbf{H}\cdot\overleftrightarrow{\chi}_o\cdot\mathbf{H} = -\frac{\hbar^2\lambda_{so}^2 s^2}{2\mu_B^2}\hat{\Omega}\cdot\overleftrightarrow{\chi}_o\cdot\hat{\Omega}. \tag{6}$$

The anisotropy energy tensor is thus at least on the order of $\lambda_{so}^2$. For a ferromagnet with cubic symmetry the rank-2 tensor $\overleftrightarrow{\chi}_o$ is isotropic and one has to go to the 4th order in $\lambda_{so}$. But for $Mn_3Ir$ the local symmetry with respect to a Mn atom is not cubic, and as discussed above $\chi_o^{xx} = \chi_o^{yy} \neq \chi_o^{zz}$. This means there is either an easy axis (along $\hat{z}$) or an easy-plane (in $xy$ plane) anisotropy. For $Mn_3Ir$ it is the former. Since the antiferromagnetic nearest neighbor coupling between Mn moments prefer a coplanar arrangement of the moments, which is incompatible with the local easy axes, the local Mn moments have to cant out-of-plane. The amount of canting is proportional to the ratio between the anisotropy energy and the nearest neighbor exchange coupling. Thus the spin canting has to be at least $\propto \lambda_{so}^2$.

## DEPENDENCE OF ORBITAL MAGNETIZATION ON RIGID ROTATIONS OF THE NONCOLLINEAR ORDER PARAMETER OF $Mn_3Ir$

Our SDFT formalism for discussing field-induced switching is formally equivalent to the LLG equation in the slow dynamics limit, which becomes a torque balance equation. A major difference between our approach and the conventional LLG-based method is how the effective fields or torques are evaluated. To use the LLG equation, a usual practice is to consider a classical Heisenberg-like model, with the Heisenberg and anisotropic exchange couplings, anisotropies, and coupling to external fields, narrowed down using symmetry and fitted to experimental data. Our method does not rely on the assumption of a Heisenberg-like classical spin model, and provides the quantities appearing in the balance equation from microscopic calculations. In particular, since the orbital-spin susceptibility appearing in the balance equation is proportional to spin-orbit coupling, which we have shown in the 1st part of the paper, the effective g-tensors of AHE AFMs with a dominant orbital magnetization can be strongly dependent on order parameter directions, which is not usually considered in phenomenological spin models.

To show this more explicitly we have calculated the dependence of the orbital magnetization of $Mn_3Ir$ on rigid rotation of the three-sublattice spin moments using SDFT. The calculation is done by first performing a scalar-relativistic self-consistent calculation so that the three local moments in a unit cell can be coplanar with respect to any initially chosen plane. Then the wavefunctions and charge densities are fed to a non-self-consistent, fully relativistic calculation which gives the orbital magnetization and the anisotropy energy. We considered two rotation axes: (111) and $(1\bar{1}0)$. The latter is equivalent to $(10\bar{1})$ used in Fig. 3 of the main text. The final states correspond to two equivalent (111) directions, obtained by rotating around the two axes by 180 and 109.47 degrees, respectively. For the rotation around (111), the orbital magnetization is always parallel with the (111) axis. So its projection onto (111) shows both its size and orientation. One can see that in this case the orbital magnetization first vanishes at 90 degrees, and then increase from zero in the opposite direction, which is another example of the nontrivial differences between noncollinear and collinear order parameters. Moreover, the strong dependence of the orbital magnetization size on rotation angle confirms our statement above.

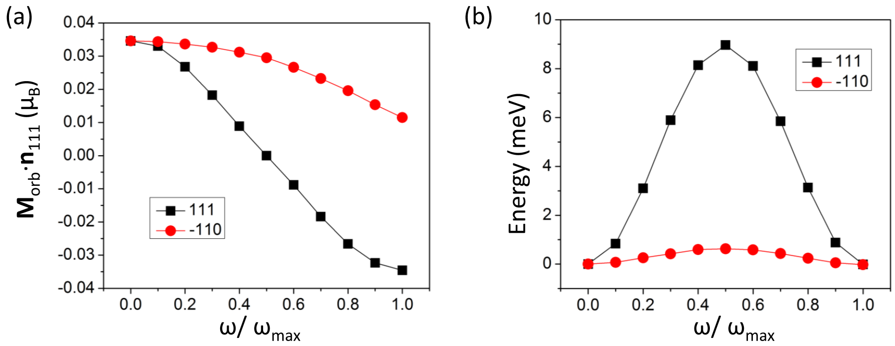


FIG. 4: (a) Orbital magnetization projected to the (111) direction, and (b) anisotropy energy versus rigid rotation of the spin order parameter of $Mn_3Ir$. The initial configuration is that the three Mn moments are coplanar in the (111) plane. The largest rotation angle $\omega_{max} = 180^\circ$ and $\arccos(-1/3) \approx 109.47^\circ$ for rotations around (111) and $(\bar{1}10)$, respectively.

## ENSEMBLE DEPENDENCE OF MAGNETIC SUSCEPTIBILITY

When talking about the magnetization of a given material, we are usually thinking of the canonical ensemble, i.e., the system has fixed particle number $N$, volume $V$, and temperature $T$. The thermodynamic potential for the canonical ensemble is the Helmholtz free energy $F(N, V, T, \boldsymbol{H})$, where $\boldsymbol{H}$ is the magnetic field strength. The magnetization is defined as

$$\boldsymbol{M}(N, V, T, \boldsymbol{H}) = -\frac{\partial F}{\partial \boldsymbol{H}}. \tag{7}$$

In statistical mechanics, the Helmholtz free energy is expressed using the partition function $Z$ through

$$F = -\frac{1}{\beta} \ln Z, \tag{8}$$

where $1/\beta = k_B T$ and $Z$ is defined as

$$Z = \mathrm{Tr}_N(e^{-\beta \hat{H}}), \tag{9}$$

where $\hat{H}$ is the Hamiltonian of the system and the trace is taken over the Hilbert space of *fixed particle number* $N$. However, in practice it is usually difficult to explicitly construct this Hilbert space and to take the trace. In contrast, it is easier to deal with the system with indefinite number of particles but a fixed chemical potential $\mu$, i.e., systems in the grand canonical ensemble, whose thermodynamic potential is the grand canonical potential $\Omega(\mu, V, T, \boldsymbol{H})$ and is related to the Helmholtz free energy through

$$\Omega = F - \mu N. \tag{10}$$

In statistical mechanics $\Omega$ is expressed using the grand partition function $\mathcal{Z}$ by

$$\Omega = -\frac{1}{\beta} \ln \mathcal{Z}, \tag{11}$$

where

$$\mathcal{Z} = \mathrm{Tr}_\mu \left[ e^{-\beta(\hat{H} - \mu \hat{N})} \right]. \tag{12}$$

It is important to recognize that $\boldsymbol{M}$ is a state variable of a thermodynamic system that is conjugate to $\boldsymbol{H}$. Thus by definition $\boldsymbol{M}$ in the grand canonical ensemble is written as

$$\boldsymbol{M}'(\mu, V, T, \boldsymbol{H}) = -\frac{\partial \Omega}{\partial \boldsymbol{H}}. \tag{13}$$

Moreover, also because $\boldsymbol{M}$ is a thermodynamic state variable, its forms in different ensembles can be trivially related to one another through change of variables, e.g.

$$\boldsymbol{M}(N, V, T, \boldsymbol{H}) = \boldsymbol{M}'(\mu(N), V, T, \boldsymbol{H}). \tag{14}$$

Therefore we only need to calculate $\boldsymbol{M}'$ once using the grand canonical ensemble.

In contrast, the definition of magnetic susceptibility (or other derivatives of state variables, such as the heat capacity) is ensemble dependent. In the grand canonical ensemble it is defined as

$$\chi_\mu \equiv \left( \frac{\partial \boldsymbol{M}'}{\partial \boldsymbol{H}} \right)_{\mu, V, T, \boldsymbol{H}} = -\frac{\partial^2 \Omega}{\partial \boldsymbol{H}^2}. \tag{15}$$

However, in the canonical ensemble it is defined as

$$\chi_N \equiv \left( \frac{\partial \boldsymbol{M}}{\partial \boldsymbol{H}} \right)_{N, V, T, \boldsymbol{H}} = -\frac{\partial^2 F}{\partial \boldsymbol{H}^2}. \tag{16}$$

The relation between $\chi_\mu$ and $\chi_N$ can be obtained in a way similar to relating $C_p$ to $C_V$:

$$\chi_N = \chi_\mu + \left( \frac{\partial \boldsymbol{M}'}{\partial \mu} \right)_{\boldsymbol{H}} \left( \frac{\partial \mu}{\partial \boldsymbol{H}} \right)_N. \tag{17}$$

Moreover, $\left( \frac{\partial \mu}{\partial \boldsymbol{H}} \right)_N$ can be calculated with the help of the Berry curvature modified density of states:

$$N = \sum_l f(\epsilon_l - \mu) = \sum_l \left( 1 + \frac{e}{\hbar} \boldsymbol{B} \cdot \boldsymbol{\Omega}_l \right) f(\epsilon_l - \boldsymbol{m}_l \cdot \boldsymbol{B} - \mu - \delta\mu), \tag{18}$$

where $l$ labels both band and wave vector of a state, $f$ is the Fermi-Dirac distribution function, $e = |e|$ is the absolute value of the electron charge, and $\boldsymbol{m}_l = \langle l | \boldsymbol{m} | l \rangle$, with

$$\boldsymbol{m} = -\frac{1}{2} \boldsymbol{j} \times \boldsymbol{r} + \frac{g\mu_B}{2} \boldsymbol{\sigma}. \tag{19}$$

Therefore

$$\left( \frac{\partial \mu}{\partial \boldsymbol{B}} \right)_N = \frac{\sum_l \left[ \frac{e}{\hbar} \boldsymbol{\Omega}_l f - \frac{\partial f}{\partial \epsilon_l} \boldsymbol{m}_l \right]}{\sum_l \frac{\partial f}{\partial \epsilon_l}}. \tag{20}$$

## DERIVATION OF THE ORBITAL-SPIN SUSCEPTIBILITY

### Perturbation theory for the quantum grand canonical potential

The grand partition function Eq. 12 has a form similar to the quantum propagator, and can indeed be treated as a propagator in the imaginary time through Wick rotation $it \to \tau$. There is a well established way to express the grand partition function of a fermionic system as a field path integral for fermion coherent states [15]:

$$\mathcal{Z} = \int D[\bar{\psi},\psi] e^{-S[\bar{\psi},\psi]}, \tag{21}$$
$$S[\bar{\psi},\psi] = \int_0^\beta d\tau \left[\bar{\psi}\partial_\tau\psi + H(\bar{\psi},\psi) - \mu N(\bar{\psi},\psi)\right],$$

where

$$D[\bar{\psi},\psi] = \lim_{N\to\infty}\prod_{n=1}^{N} d\bar{\psi}_n d\psi_n, \tag{22}$$

and the fields $\bar{\psi}$, $\psi$ satisfy the boundary condition

$$\bar{\psi}(0) = -\bar{\psi}(\beta),\ \ \psi(0) = -\psi(\beta). \tag{23}$$

If we assume that the Hamiltonian is quadratic in the fields $\bar{\psi},\psi$, which is valid for noninteracting systems, we can obtain $\mathcal{Z}$ using Gaussian integration as

$$\mathcal{Z} = \det\left[\beta\left(\partial_\tau + \hat{H} - \mu\hat{N}\right)\right] = \det\left[\beta\left(-i\hat{\omega} + \hat{H} - \mu\hat{N}\right)\right] \equiv \det\left[\beta\hat{G}^{-1}\right], \tag{24}$$

where $\hat{G}$ is the thermal Green's function. We thus have

$$\Omega = -\frac{1}{\beta}\ln\mathcal{Z} = -\frac{1}{\beta}\ln\det\left[\beta\hat{G}^{-1}\right] = -\frac{1}{\beta}\mathrm{Tr}\ln\left[\beta\hat{G}^{-1}\right]. \tag{25}$$

Assuming that $H = H_0 + \delta H$, where $\delta H$ is a perturbation, we only need to modify Eq. 25 as

$$\begin{aligned}\Omega &= -\frac{1}{\beta}\mathrm{Tr}\ln\left[\beta\left(\hat{G}_0^{\ -1} + \delta\hat{H}\right)\right] = \Omega_0 - \frac{1}{\beta}\mathrm{Tr}\ln\left[\hat{1} + \hat{G}_0\delta\hat{H}\right] \\ &= \Omega_0 - \frac{1}{\beta}\sum_{m=1}^{\infty}\frac{(-1)^{m+1}}{m}\mathrm{Tr}\left[\left(\hat{G}_0\delta\hat{H}\right)^m\right],\end{aligned} \tag{26}$$

and to calculate e.g. $\chi_\mu$, we only need to keep the $m = 2$ term in Eq. 26. More explicitly, if $\delta H$ is independent of $\tau$,

$$\Omega^{(2)} = \frac{1}{2\beta}\mathrm{Tr}\left[\hat{G}_0\delta\hat{H}\hat{G}_0\delta\hat{H}\right] = \frac{1}{2\beta}\sum_n (G_0)_{n,ab}(\delta H)_{bc}(G_0)_{n,cd}(\delta H)_{da}, \tag{27}$$

where summation over repeated indices $a, b, c, d$ is assumed.

### Perturbation Hamiltonian

A uniform magnetic field can be obtained by taking the $q \to 0$ limit of the following periodic vector potential[16, 17]

$$\boldsymbol{A}(\boldsymbol{r}) = \frac{\boldsymbol{B}_0\times\boldsymbol{q}}{2iq^2}\left(e^{i\boldsymbol{q}\cdot\boldsymbol{r}} - e^{-i\boldsymbol{q}\cdot\boldsymbol{r}}\right),\ \ \boldsymbol{q}\cdot\boldsymbol{B} = 0, \tag{28}$$
$$\boldsymbol{B}(\boldsymbol{r}) = \nabla\times\boldsymbol{A} = \frac{\boldsymbol{B}_0}{2}\left(e^{i\boldsymbol{q}\cdot\boldsymbol{r}} + e^{-i\boldsymbol{q}\cdot\boldsymbol{r}}\right),$$

which enters the Hamiltonian through the substitution

$$c_{i\alpha} \to c_{i\alpha}\exp\left[\frac{ie}{\hbar}\int_0^i \boldsymbol{A}\cdot d\boldsymbol{r}\right], \tag{29}$$

where the starting point of the integral in the exponent is arbitrary. Thus for a quadratic Hamiltonian $H = \sum_{ij,\alpha\beta} h_{ij}^{\alpha\beta} c_{i\alpha}^\dagger c_{j\beta}$ it becomes in the presence of $\boldsymbol{A}$

$$H = \sum_{ij,\alpha\beta} h_{ij}^{\alpha\beta} \exp\left[-\frac{ie}{\hbar}\int_j^i \boldsymbol{A}\cdot d\boldsymbol{r}\right] c_{i\alpha}^\dagger c_{j\beta}. \tag{30}$$

For small $\boldsymbol{A}$ we can expand the exponent and obtain the perturbation Hamiltonian

$$\delta H = \sum_{ij,\alpha\beta} h_{ij}^{\alpha\beta}\left[-\frac{ie}{\hbar}\boldsymbol{A}\left(\frac{\boldsymbol{r}_i+\boldsymbol{r}_j}{2}\right)\cdot\ (\boldsymbol{r}_i-\boldsymbol{r}_j)\right] c_{i\alpha}^\dagger c_{j\beta}. \tag{31}$$

which under Fourier transform becomes

$$\begin{aligned}\delta H &= -\sum_{\boldsymbol{k}\boldsymbol{q},\alpha\beta} c_{\boldsymbol{k}^+\alpha}^\dagger c_{\boldsymbol{k}^-\beta}\left(-\frac{e}{\hbar}\partial_{\boldsymbol{k}} h_{\boldsymbol{k}}^{\alpha\beta}\right)\cdot \boldsymbol{A}_{\boldsymbol{q}} \\ &\equiv -\sum_{\boldsymbol{q}} \boldsymbol{j}_{-\boldsymbol{q}}\cdot\boldsymbol{A}_{\boldsymbol{q}}.\end{aligned} \tag{32}$$

In the equations above $\boldsymbol{k}^\pm = \boldsymbol{k} \pm \frac{\boldsymbol{q}}{2}$.

For the present problem in which $A$ only has two Fourier components, the perturbation Hamiltonian due to the vector potential is

$$\delta H_A = -\boldsymbol{j}_{-\boldsymbol{q}}\cdot\boldsymbol{A}_q - \boldsymbol{j}_{\boldsymbol{q}}\cdot\boldsymbol{A}_{-q}, \tag{33}$$

where $\boldsymbol{A}_{\boldsymbol{q}} = \frac{\boldsymbol{B}_0\times\boldsymbol{q}}{2iq^2}$.

In addition, since we are interested in the orbital-spin crossed part of the susceptibility, we need to consider a Zeeman field $\boldsymbol{B}^s$ coupled to the spin degree of freedom only

$$\begin{aligned}\delta H_B &= -\sum_{i\alpha\beta} c_{i\alpha}^\dagger c_{i\beta}\frac{g\mu_B}{2}\boldsymbol{\sigma}^{\alpha\beta}\cdot\boldsymbol{B}^s(\boldsymbol{r}_i) \\ &= -\sum_{\boldsymbol{k}\boldsymbol{q},\alpha\beta} c_{\boldsymbol{k}^+\alpha}^\dagger c_{\boldsymbol{k}^-\beta}\frac{g\mu_B}{2}\boldsymbol{\sigma}^{\alpha\beta}\cdot\boldsymbol{B}_{\boldsymbol{q}}^s \equiv -\sum_{\boldsymbol{q}} \boldsymbol{m}_{-\boldsymbol{q}}^s\cdot\boldsymbol{B}_{\boldsymbol{q}}^s.\end{aligned} \tag{34}$$

Note that the matrix elements of the spin operator is independent of $\boldsymbol{k}$. We have adopted the convention that $g \approx -2$, which is convenient when we need to change the magnetic field to an exchange field later. Since $\boldsymbol{B}^s(\boldsymbol{r})$ is real we also have $\boldsymbol{B}_{\boldsymbol{q}}^s = \boldsymbol{B}_{-\boldsymbol{q}}^{s*}$

### Green's function formula of the orbital-spin susceptibility

We can now use Eq. 27 to calculate the 2nd order term of the grand canonical potential, where $\delta H = \delta H_A + \delta H_B$ is given by Eq. 33 and 34. To calculate the trace in Eq. 27, we note that since $G_0$ is diagonal in $\boldsymbol{k}$, the 2nd (1st) momentum subscript of the first $\delta H$ in Eq. 27 must be the same as the 1st (2nd) momentum subscript of the second $\delta H$. We thus arrive at

$$\Omega^{(2)} = \frac{1}{\beta}\sum_n\int[d\boldsymbol{k}]G_0^{ab}(\omega_n,\boldsymbol{k})(\boldsymbol{j}_{\boldsymbol{k}^+}\cdot\boldsymbol{A}_{-\boldsymbol{q}} + \boldsymbol{m}^s\cdot\boldsymbol{B}_{-\boldsymbol{q}}^s)^{bc}G_0^{cd}(\omega_n,\boldsymbol{k}+\boldsymbol{q})(\boldsymbol{j}_{\boldsymbol{k}^+}\cdot\boldsymbol{A}_{\boldsymbol{q}} + \boldsymbol{m}^s\cdot\boldsymbol{B}_{\boldsymbol{q}}^s)^{da}, \tag{35}$$

where

$$\begin{aligned}\boldsymbol{j}_{\boldsymbol{k}}^{ab} &\equiv -\frac{e}{\hbar}\partial_{\boldsymbol{k}} h_{\boldsymbol{k}}^{ab} = -e\boldsymbol{v}_{\boldsymbol{k}}^{ab}, \\ (\boldsymbol{m}^s)^{ab} &= \frac{g\mu_B}{2}\boldsymbol{\sigma}^{ab}.\end{aligned} \tag{36}$$

We are only interested in the crossed term in $\Omega^{(2)}$, which is

$$\begin{aligned}\Omega_{AB}^{(2)} = \frac{1}{\beta}\sum_n\int[d\boldsymbol{k}]^\beta \mathrm{tr}\big[&A_{\boldsymbol{q}}^\alpha B_{\boldsymbol{q}}^{s\beta*}G_0(\omega_n,\boldsymbol{k})m_s^\beta G_0(\omega_n,\boldsymbol{k}+\boldsymbol{q})j_{\boldsymbol{k}^+}^\alpha \\ &-A_{\boldsymbol{q}}^\alpha B_{\boldsymbol{q}}^{s\beta}G_0(\omega_n,\boldsymbol{k})j_{\boldsymbol{k}^+}^\alpha G_0(\omega_n,\boldsymbol{k}+\boldsymbol{q})m_s^\beta\big],\end{aligned} \tag{37}$$

in which we have used $\boldsymbol{A}_{-\boldsymbol{q}} = -\boldsymbol{A}_{\boldsymbol{q}}$. To get a finite value when $q \to 0$ we need to expand the trace in $\Omega^{(2)}_{AB}$ to linear order in $\boldsymbol{q}$. We do this by making use of the following relation

$$\partial_{\boldsymbol{k}} G_0(\boldsymbol{k}) = -G_0(\boldsymbol{k})\hbar \boldsymbol{v}_{\boldsymbol{k}} G_0(\boldsymbol{k}). \tag{38}$$

Keeping only the linear in $q$ terms in the trace, we get

$$\Omega^{(2)}_{AB} = \frac{e\hbar g\mu_B}{2\beta}\sum_n \int [d\boldsymbol{k}](A^\alpha_{\boldsymbol{q}} q^\gamma)\mathrm{tr}\left[B^{s\beta *}_{\boldsymbol{q}} G_0 v^\gamma G_0 v^\alpha G_0 \sigma^\beta - B^{s\beta}_{\boldsymbol{q}} G_0 v^\alpha G_0 v^\gamma G_0 \sigma^\beta\right]. \tag{39}$$

Note that we did not expand $\boldsymbol{j}_{\boldsymbol{k}+}$ in powers of $\boldsymbol{q}$, the reason of which will become clear below. Also all the Green's functions and operators in the equation above are at momentum $\boldsymbol{k}$.

Now we take a closer look at the factor $A^\alpha_{\boldsymbol{q}} q^\gamma$

$$A^\alpha_{\boldsymbol{q}} q^\gamma = \frac{\epsilon_{\alpha\mu\nu} B^\mu_0 q^\nu q^\gamma}{2iq^2} \tag{40}$$

Since $\boldsymbol{q}$ can point to any direction in the plane perpendicular to $\boldsymbol{B}_0$, we need to take an angular average of the product $q^\nu q^\gamma$: $\langle q^\nu q^\gamma\rangle_\phi = \frac{1}{2}q^2\delta^{\nu\gamma}$. Therefore

$$\langle A^\alpha_{\boldsymbol{q}} q^\gamma\rangle_\phi = \frac{\epsilon_{\mu\gamma\alpha} B^\mu_0}{4i}. \tag{41}$$

It is also clear now why we do not need to expand $j^\alpha_{\boldsymbol{k}+}$ in $q^\gamma$, since $\epsilon_{\mu\gamma\alpha}\partial_\gamma\partial_\alpha h_{\boldsymbol{k}} = 0$. Collecting all terms, we finally arrive at

$$\Omega^{(2)}_{AB} = B^\mu_0 B^\beta_s \frac{e\hbar g\mu_B \epsilon_{\mu\gamma\alpha}}{4i\beta}\sum_n \int [d\boldsymbol{k}]\mathrm{tr}\left[G_0 v^\gamma G_0 v^\alpha G_0 \sigma^\beta\right], \tag{42}$$

where $\boldsymbol{B}_s \equiv \lim_{q\to 0}\mathrm{Re}(\boldsymbol{B}^s_{\boldsymbol{q}})$ represents an uniform Zeeman field. The orbital-spin susceptibility is therefore

$$\chi^{\alpha\beta}_{os} = -\frac{\partial^2\Omega}{\partial B^\alpha_0 \partial B^\beta_s} = i\frac{e\hbar g\mu_B \epsilon_{\alpha\gamma\delta}}{4\beta}\sum_n \int [d\boldsymbol{k}]\mathrm{tr}\left[G_0 v^\gamma G_0 v^\delta G_0 \sigma^\beta\right], \tag{43}$$

where $B_0$ and $B_s$ respectively means the magnetic field that enters the Hamiltonian through orbital and spin coupling.

### Orbital-spin susceptibility formula suitable for model calculations

We would like to convert Eq. 43 to a form more suitable for model or DFT calculations. To this end we calculate the quantity

$$\Pi \equiv \frac{1}{\beta}\epsilon_{\alpha\gamma\delta}\sum_{n\boldsymbol{k}}\mathrm{tr}\left[G_0 v^\gamma G_0 v^\delta G_0 \sigma^\beta\right]. \tag{44}$$

In the eigenstate basis of $H_0$, $\Pi$ can be separated into the following parts:

$$\Pi = \frac{1}{\beta}\epsilon_{\alpha\gamma\delta}\sum_{n\boldsymbol{k}} v^\gamma_{ab} v^\delta_{bc}\sigma^\beta_{ca} G_a G_b G_c = \Pi_1 + \Pi_2 + \Pi_3 + \Pi_4 + \Pi_5, \tag{45}$$

$$\Pi_1 = \frac{1}{\beta}\epsilon_{\alpha\gamma\delta}\sum_{n\boldsymbol{k}} v^\gamma_{aa} v^\delta_{aa}\sigma^\beta_{aa} G^3_a = 0,$$

$$\Pi_2 = \frac{1}{\beta}\epsilon_{\alpha\gamma\delta}\sum_{n\boldsymbol{k}} v^\gamma_{aa} v^\delta_{ac}\sigma^\beta_{ca} G^2_a G_c = \frac{1}{\beta}\epsilon_{\alpha\gamma\delta}\sum_{n\boldsymbol{k}} v^\gamma_{aa} v^\delta_{ab}\sigma^\beta_{ba} G^2_a G_b,\ a \neq b,$$

$$\Pi_3 = \frac{1}{\beta}\epsilon_{\alpha\gamma\delta}\sum_{n\boldsymbol{k}} v^\gamma_{ab} v^\delta_{bb}\sigma^\beta_{ba} G_a G^2_b = \frac{1}{\beta}\epsilon_{\alpha\gamma\delta}\sum_{n\boldsymbol{k}} v^\gamma_{ba} v^\delta_{aa}\sigma^\beta_{ab} G^2_a G_b,\ a \neq b,$$

$$\Pi_4 = \frac{1}{\beta}\epsilon_{\alpha\gamma\delta}\sum_{n\boldsymbol{k}} v^\gamma_{ab} v^\delta_{ba}\sigma^\beta_{aa} G^2_a G_b,\ a \neq b,$$

$$\Pi_5 = \frac{1}{\beta}\epsilon_{\alpha\gamma\delta}\sum_{n\boldsymbol{k}} v^\gamma_{ab} v^\delta_{bc}\sigma^\beta_{ca} G_a G_b G_c,\ a \neq b \neq c \neq a,$$

Where we have omitted the subscript 0 of Green's function of the unperturbed Hamiltonian. $\Pi_1 = 0$ because of the $\epsilon_{\alpha\gamma\delta}$ factor. Below we calculate $\Pi_2 - \Pi_5$ separately.

In the $H_0$ eigenstate basis we have

$$G_a = \frac{1}{-i\omega_n + \epsilon_a - \mu}. \tag{46}$$

Therefore

$$\partial_{\epsilon_a} G_a = -\frac{1}{(-i\omega_n + \epsilon_a - \mu)^2} = -G_a^2, \tag{47}$$

which leads to

$$\begin{aligned} \Pi_2 &= -\frac{1}{\beta}\epsilon_{\alpha\gamma\delta}\partial_{\epsilon_a}\left[\sum_{n\boldsymbol{k}} v^\gamma_{aa} v^\delta_{ab} \sigma^\beta_{ba} G_a G_b\right] \\ &= -\epsilon_{\alpha\gamma\delta}\sum_{\boldsymbol{k}} v^\gamma_{aa} v^\delta_{ab}\sigma^\beta_{ba}\left(\frac{f'_a}{E_{ab}} - \frac{f_a - f_b}{E^2_{ab}}\right) \end{aligned} \tag{48}$$

where $f'_a \equiv \partial_{\epsilon_a} f(\epsilon_a - \mu)$ and $E_{ab} = \epsilon_a - \epsilon_b$.

Similarly we can obtain

$$\begin{aligned} \Pi_3 &= -\epsilon_{\alpha\gamma\delta}\sum_{\boldsymbol{k}} v^\gamma_{ba} v^\delta_{aa}\sigma^\beta_{ab}\left(\frac{f'_a}{E_{ab}} - \frac{f_a - f_b}{E^2_{ab}}\right), \\ \Pi_4 &= -\epsilon_{\alpha\gamma\delta}\sum_{\boldsymbol{k}} v^\gamma_{ab} v^\delta_{ba}\sigma^\beta_{aa}\left(\frac{f'_a}{E_{ab}} - \frac{f_a - f_b}{E^2_{ab}}\right), \end{aligned} \tag{49}$$

and for $\Pi_5$ the Matsubara summation can be trivially done since there are only simple poles

$$\begin{aligned} \Pi_5 &= -\epsilon_{\alpha\gamma\delta}\sum_{\boldsymbol{k}} v^\gamma_{ab} v^\delta_{bc}\sigma^\beta_{ca}\left(\frac{f_a}{E_{ab}E_{ac}} + \frac{f_b}{E_{ba}E_{bc}} + \frac{f_c}{E_{ca}E_{cb}}\right) \\ &= -\epsilon_{\alpha\gamma\delta}\sum_{\boldsymbol{k}} \frac{f_a}{E_{ab}E_{ac}}\left(v^\gamma_{ab} v^\delta_{bc}\sigma^\beta_{ca} + v^\gamma_{ba} v^\delta_{ac}\sigma^\beta_{cb} + v^\gamma_{cb} v^\delta_{ba}\sigma^\beta_{ac}\right). \end{aligned} \tag{50}$$

Eqs. 48, 49, 50 are already suitable for model calculations. However, it is sometimes more convenient to convert $f'_a$ into $f_a$ through partial integration so that one does not have to deal with delta functions at zero temperature. We would also like to compare our results with that in [13, 14]. To this end we first prove the following identity (Eq. E3 in [13])

$$\frac{1}{2}\epsilon_{\alpha\gamma\delta}\sum_{\boldsymbol{k}} \frac{f'_a}{E_{ab}}(v^\gamma_{ab}\sigma^\beta_{ba}v^\delta_{aa} - \sigma^\beta_{ab}v^\gamma_{ba}v^\delta_{aa}) = \epsilon_{\alpha\gamma\delta}\sum_{\boldsymbol{k}}\left(\frac{v^\delta_{ab}\sigma^\beta_{bc}v^\gamma_{ca}}{E_{ab}E_{ac}} + \frac{v^\gamma_{ab}v^\delta_{ba}\sigma^\beta_{aa}}{E^2_{ab}}\right) f_a. \tag{51}$$

Note that in the first term on the right hand side we allow $b = c$, even though $a \neq b, a \neq c$.

We start from the left hand side of Eq. 51

$$\begin{aligned} &\frac{1}{2}\epsilon_{\alpha\gamma\delta}\sum_{\boldsymbol{k}} \frac{f'_a}{E_{ab}}(v^\gamma_{ab}\sigma^\beta_{ba}v^\delta_{aa} - \sigma^\beta_{ab}v^\gamma_{ba}v^\delta_{aa}) = \frac{1}{2\hbar}\epsilon_{\alpha\gamma\delta}\sum_{\boldsymbol{k}}\frac{\partial_\delta f_a}{E_{ab}}(v^\gamma_{ab}\sigma^\beta_{ba} - \sigma^\beta_{ab}v^\gamma_{ba}) \\ &= -\frac{1}{2\hbar}\epsilon_{\alpha\gamma\delta}\sum_{\boldsymbol{k}} f_a\partial_\delta\left(\frac{v^\gamma_{ab}\sigma^\beta_{ba} - \sigma^\beta_{ab}v^\gamma_{ba}}{E_{ab}}\right) \\ &= (1) + (2), \end{aligned} \tag{52}$$

where

$$(1) = \frac{1}{2}\epsilon_{\alpha\gamma\delta}\sum_{\boldsymbol{k}} \frac{f_a}{E^2_{ab}}(v^\delta_{aa} - v^\delta_{bb})(v^\gamma_{ab}\sigma^\beta_{ba} - \sigma^\beta_{ab}v^\gamma_{ba}), \tag{53}$$

and

$$
\begin{aligned}
(2) &= -\frac{1}{2}\epsilon_{\alpha\gamma\delta}\sum_{\boldsymbol{k}}\frac{f_a}{E_{ab}}\left(\frac{v^{\delta}_{ac}v^{\gamma}_{cb}\sigma^{\beta}_{ba}}{E_{ac}}+\frac{v^{\gamma}_{ac}v^{\delta}_{cb}\sigma^{\beta}_{ba}}{E_{bc}}+\frac{v^{\gamma}_{ab}v^{\delta}_{bc}\sigma^{\beta}_{ca}}{E_{bc}}+\frac{v^{\gamma}_{ab}\sigma^{\beta}_{bc}v^{\delta}_{ca}}{E_{ac}}-a\leftrightarrow b\right) \\
&= (2)'+(2)'',
\end{aligned} \tag{54}
$$

in which we have used $\partial_\delta|u_{a\boldsymbol{k}}\rangle=\sum_{b\neq a}\frac{\hbar v^{\delta}_{ba}}{E_{ab}}|u_{b\boldsymbol{k}}\rangle$. $(2)'$ is a collection of terms in (2) that have the two subscripts not constrained by the energy difference denominators equal to each other:

$$
\begin{aligned}
(2)' &= -\frac{1}{2}\epsilon_{\alpha\gamma\delta}\sum_{\boldsymbol{k}}\frac{f_a}{E^2_{ab}}\left(v^{\delta}_{ab}v^{\gamma}_{bb}\sigma^{\beta}_{ba}-v^{\gamma}_{aa}v^{\delta}_{ab}\sigma^{\beta}_{ba}-v^{\gamma}_{ab}v^{\delta}_{ba}\sigma^{\beta}_{aa}+v^{\gamma}_{ab}\sigma^{\beta}_{bb}v^{\delta}_{ba}+a\leftrightarrow b\right) \\
&= \frac{1}{2}\epsilon_{\alpha\gamma\delta}\sum_{\boldsymbol{k}}\frac{f_a}{E^2_{ab}}\left[(v^{\gamma}_{aa}-v^{\gamma}_{bb})(v^{\delta}_{ab}\sigma^{\beta}_{ba}-v^{\delta}_{ba}\sigma^{\beta}_{ab})+(\sigma^{\beta}_{aa}-\sigma^{\beta}_{bb})(v^{\gamma}_{ab}v^{\delta}_{ba}-v^{\gamma}_{ba}v^{\delta}_{ab})\right].
\end{aligned} \tag{55}
$$

The first term of $(2)'$ cancels (1) because of the $\epsilon_{\alpha\gamma\delta}$ factor. Therefore

$$
(1)+(2)'=\epsilon_{\alpha\gamma\delta}\sum_{\boldsymbol{k}}\frac{f_a}{E^2_{ab}}(\sigma^{\beta}_{aa}-\sigma^{\beta}_{bb})v^{\gamma}_{ab}v^{\delta}_{ba}. \tag{56}
$$

We now turn to $(2)''$. Using the antisymmetry of $\gamma,\delta$ we can combine the first two terms in the parentheses:

$$
\begin{aligned}
(2)'' &= -\frac{1}{2}\epsilon_{\alpha\gamma\delta}\sum_{\boldsymbol{k}}\frac{f_a}{E_{ab}}\left[\frac{v^{\delta}_{ac}v^{\gamma}_{cb}\sigma^{\beta}_{ba}}{E_{ac}E_{bc}}(-E_{ab})+\frac{v^{\gamma}_{ab}v^{\delta}_{bc}\sigma^{\beta}_{ca}}{E_{bc}}+\frac{v^{\gamma}_{ab}\sigma^{\beta}_{bc}v^{\delta}_{ca}}{E_{ac}}-a\leftrightarrow b\right] \\
&= \frac{1}{2}\epsilon_{\alpha\gamma\delta}\sum_{\boldsymbol{k}}\frac{f_a}{E_{ac}E_{bc}}(v^{\delta}_{ac}v^{\gamma}_{cb}\sigma^{\beta}_{ba}+a\leftrightarrow b)-\frac{f_a}{E_{ab}}\left(\frac{v^{\gamma}_{ab}v^{\delta}_{bc}\sigma^{\beta}_{ca}}{E_{bc}}+\frac{v^{\gamma}_{ab}\sigma^{\beta}_{bc}v^{\delta}_{ca}}{E_{ac}}-a\leftrightarrow b\right).
\end{aligned} \tag{57}
$$

The first term in the first parentheses cancels the first term in the second parentheses after permuting $bc$ in the latter and using the antisymmetry of $\gamma,\delta$. The second term in the first parentheses cancels the 4th term in the second parentheses. The only two terms that remain can be combined by permuting $bc$ and $\gamma\delta$, which gives

$$
(2)''=\epsilon_{\alpha\gamma\delta}\sum_{\boldsymbol{k}}\frac{f_a}{E_{ab}E_{ac}}v^{\delta}_{ab}\sigma^{\beta}_{bc}v^{\gamma}_{ca}. \tag{58}
$$

Note that in $(2)''$ $a\neq b\neq c\neq a$. If we relax this constraint, the 2nd term in $(1)+(2)'$ can be absorbed in $(2)''$, and we arrive at the final result Eq. 51.

Now we use Eq. 51 to simplify $\Pi_2+\Pi_3$:

$$
\begin{aligned}
\Pi_2+\Pi_3 &= \epsilon_{\alpha\gamma\delta}\sum_{\boldsymbol{k}}\left[v^{\delta}_{aa}(v^{\gamma}_{ab}\sigma^{\beta}_{ba}-v^{\gamma}_{ba}\sigma^{\beta}_{ab})\frac{f'_a}{E_{ab}}+(v^{\gamma}_{aa}+v^{\gamma}_{bb})(v^{\delta}_{ab}\sigma^{\beta}_{ba}-v^{\delta}_{ba}\sigma^{\beta}_{ab})\frac{f_a}{E^2_{ab}}\right] \\
&= \epsilon_{\alpha\gamma\delta}\sum_{\boldsymbol{k}}f_a\left[2\frac{v^{\delta}_{ab}\sigma^{\beta}_{bc}v^{\gamma}_{ca}}{E_{ab}E_{ac}}+2\frac{v^{\gamma}_{ab}v^{\delta}_{ba}\sigma^{\beta}_{aa}}{E^2_{ab}}+\frac{(v^{\gamma}_{aa}+v^{\gamma}_{bb})(v^{\delta}_{ab}\sigma^{\beta}_{ba}-v^{\delta}_{ba}\sigma^{\beta}_{ab})}{E^2_{ab}}\right].
\end{aligned} \tag{59}
$$

Note that the first term on the right hand side includes the case of $b=c$.

$\Pi_4$ can be rewritten as the following

$$
\Pi_4=\epsilon_{\alpha\gamma\delta}\sum_{\boldsymbol{k}}\left[-f'_a\frac{v^{\gamma}_{ab}v^{\delta}_{ba}\sigma^{\beta}_{aa}}{E_{ab}}+\frac{f_a}{E^2_{ab}}(v^{\gamma}_{ab}v^{\delta}_{ba}\sigma^{\beta}_{aa})-\frac{f_a}{E^2_{ab}}(v^{\gamma}_{ba}v^{\delta}_{ab}\sigma^{\beta}_{bb})\right] \tag{60}
$$

We now combine terms in $\Pi_2+\Pi_3$ (Eq. 59), $\Pi_4$ (Eq. 60), and $\Pi_5$ (Eq. 50) in the following way: The last term in Eq. 60 can be absorbed into the 2nd term in Eq. 50 (after permuting $bc$), if we relax the constraint in Eq. 50 of $b\neq c$, and they together cancel half of the first term in Eq. 59; the 2nd term in Eq. 59 can be combined with the 2nd term in Eq. 60; the part of the last term in Eq. 59 that is proportional to $v^{\gamma}_{bb}$ can be absorbed into the 1st and the 3rd terms in Eq. 50, if we relax the constraint of $b\neq c$. Collecting all terms, and doing a couple of permutations of $bc$ and $\gamma\delta$ when needed, we arrive at

$$
\Pi=\epsilon_{\alpha\gamma\delta}\sum_{\boldsymbol{k}}\frac{v^{\gamma}_{ab}v^{\delta}_{ba}\sigma^{\beta}_{aa}}{E_{ba}}f'_a+\left[\frac{v^{\gamma}_{aa}(v^{\delta}_{ab}\sigma^{\beta}_{ba}-v^{\delta}_{ba}\sigma^{\beta}_{ab})+3\sigma^{\beta}_{aa}v^{\gamma}_{ab}v^{\delta}_{ba}}{E^2_{ab}}-\frac{v^{\gamma}_{ab}v^{\delta}_{bc}\sigma^{\beta}_{ca}+v^{\gamma}_{ab}\sigma^{\beta}_{bc}v^{\delta}_{ca}+\sigma^{\beta}_{ab}v^{\gamma}_{bc}v^{\delta}_{ca}}{E_{ab}E_{ac}}\right]f_a. \tag{61}
$$

The final expression for $\chi_{os}$ is

$$\chi_{os}^{\alpha\beta} = i\frac{e\hbar g\mu_B}{4}\epsilon_{\alpha\gamma\delta}\sum_{\boldsymbol{k}}\frac{v_{ab}^{\gamma}v_{ba}^{\delta}\sigma_{aa}^{\beta}}{E_{ba}}f'_a$$
$$+i\frac{e\hbar g\mu_B}{4}\epsilon_{\alpha\gamma\delta}\sum_{\boldsymbol{k}}\left[\frac{v_{aa}^{\gamma}(v_{ab}^{\delta}\sigma_{ba}^{\beta}-v_{ba}^{\delta}\sigma_{ab}^{\beta})+3\sigma_{aa}^{\beta}v_{ab}^{\gamma}v_{ba}^{\delta}}{E_{ab}^2}-\frac{v_{ab}^{\gamma}v_{bc}^{\delta}\sigma_{ca}^{\beta}+v_{ab}^{\gamma}\sigma_{bc}^{\beta}v_{ca}^{\delta}+\sigma_{ab}^{\beta}v_{bc}^{\gamma}v_{ca}^{\delta}}{E_{ab}E_{ac}}\right]f_a. \tag{62}$$

Note that in the equation above $b \neq a \neq c$, but $b = c$ is allowed. The first term can be viewed as a correction/renormalization to the $g$ factor [13] and is hence separated out. But it has to be taken into account when we discuss the magnetic field induced spin-density later.

We now compare Eq. 62 with the result obtained by Misra and Kleinman using a different method (Eqs. 3.40 and 3.46 in [13]). Apart from different notations of the indices (also $\hbar\boldsymbol{v} \to \boldsymbol{\pi}$ in there), one can easily see that all the terms in Eq. 62 are identical to their counterparts in [13]. (There is a mistake in the 2nd term of their Eq. 3.46, where it should be $\pi^{\alpha}_{n\rho,m\rho'}$.) The overall prefactor including the sign is also the same (remember that $g \approx -2$ in our notation, in their paper $h_{xy} = -h_{yx} = eB/2\hbar$, and $\partial_B^2$ gives another factor of 2).

The expression of $\chi_{os}$ obtained by Misra and Kleinman is still inconvenient for numerical calculations. This is because the summation over band indices is over both occupied and unoccupied bands, except for $a$ which is restricted to filled bands. Thus the integrand will diverge at any accidental degeneracies in the Brillouin zone. To cure this pathological behavior we have to look a little more deeply into Eq. 62 and see if we can change the integrand to a smooth function of $\boldsymbol{k}$. To this end we go back to Eqs. 48, 49, 50, and consider the simple case of a band insulator. In this case we can ignore all terms proportional to $f'$ which is a $\delta$ function centered at the band gap. The remaining terms are

$$\Pi_{2-4} \equiv \Pi_2+\Pi_3+\Pi_4 = \epsilon_{\alpha\gamma\delta}\sum_{\boldsymbol{k}}\frac{f_a-f_b}{E_{ab}^2}(v_{aa}^{\gamma}v_{ab}^{\delta}\sigma_{ba}^{\beta}+v_{ba}^{\gamma}v_{aa}^{\delta}\sigma_{ab}^{\beta}+v_{ab}^{\gamma}v_{ba}^{\delta}\sigma_{aa}^{\beta}), \tag{63}$$
$$\Pi_5 = -\epsilon_{\alpha\gamma\delta}\sum_{\boldsymbol{k}}v_{ab}^{\gamma}v_{bc}^{\delta}\sigma_{ca}^{\beta}\left(\frac{f_a}{E_{ab}E_{ac}}+\frac{f_b}{E_{ba}E_{bc}}+\frac{f_c}{E_{ca}E_{cb}}\right),\ a\neq b\neq c\neq a.$$

It is then clear that $\Pi_{2-4}$ only has contributions from the matrix elements that are between two eigenstates at different sides of the gap. Thus the denominator will never vanish. Although it may not be apparent at first sight, $\Pi_5$ also has such a property. To see this we separately consider the situations of (1) $f_a = f_b = f_c$, (2) $f_a = f_b = 1$, $f_c = 0$, plus permutations of $a, b, c$, and (3) $f_a = f_b = 0$, $f_c = 1$, plus permutations of $a, b, c$. For (1) it is trivial to observe that $\frac{1}{E_{ab}E_{ac}}+\frac{1}{E_{ba}E_{bc}}+\frac{1}{E_{ca}E_{cb}}=0$. For (2) the terms in the parentheses become $-\frac{1}{E_{ac}E_{bc}}$, which will not diverge since $c$ is empty while $a$ and $b$ are filled, and other permutations of $a, b, c$ give similar results. For (3) only the last term $\frac{1}{E_{ac}E_{bc}}$ in the parentheses is nonzero, and it's not divergent since $a, b$ are empty while $c$ is filled, and other permutations give similar results. Therefore for insulators we only need to do the integrals in Eq. 63 which are well behaved in the Brillouin zone.

### Corrections to the orbital-spin susceptibility in SDFT

For completeness, in this section we comment on the self-consistent-field corrections to the orbital-spin susceptibility within SDFT, when calculating the response to a *real* Zeeman field. Note the orbital-spin susceptibility used in the main text for discussing magnetic-field-induced switching is not the response to actual Zeeman fields, but to order parameter re-orientation, for which we do not need to include such corrections. Taking into account the orbital response to both the Zeeman field and the associated change in the exchange field, we have

$$\delta\mathbf{M}_{orb} = \overleftrightarrow{\chi}_{os}\cdot\left(\mathbf{H}_{spin}+\frac{\hbar}{g\mu_B}\delta\boldsymbol{\Delta}_{ex}\right), \tag{64}$$
$$\delta\boldsymbol{\Delta}_{ex} = -\frac{\Delta_{ex}}{M_s}\overleftrightarrow{\chi}_s\cdot(\mathbf{H}_{spin}+\frac{\hbar}{g\mu_B}\delta\boldsymbol{\Delta}_{ex}),$$

where we have assumed that only the direction of the exchange field is significantly modified by the external Zeeman field. The many-body orbital-spin susceptibility within SDFT is therefore

$$\overleftrightarrow{\chi}_{os}^{SDFT} = \overleftrightarrow{\chi}_{os}\cdot\left[1-\frac{\hbar\Delta_{ex}}{g\mu_B M_s}\left(1+\frac{\hbar\Delta_{ex}}{g\mu_B M_s}\overleftrightarrow{\chi}_s\right)^{-1}\cdot\overleftrightarrow{\chi}_s\right]. \tag{65}$$

## NON-RIGID ROTATION OF NONCOLLINEAR ORDER PARAMETERS

The inverse triangular order of $Mn_3Sn$ leads to vanishing in-plane anisotropy if one only considers the uniaxial anisotropy for each magnetic sublattice. Although for more complicated symmetry-allowed anisotropy terms such a perfect cancellation may not occur, as far as this model is concerned, our assumption of rigid rotation is inadequate, since the switching barrier is zero. One can show that in this case the barrier should scale with the net spin magnetization at the saddle point of the switching process.

To generalize Eq. (6) in the main text we need to include a few more parameters $\{\omega_i\}$ besides the three characterizing the rigid body rotation $\hat{\Omega}$. These parameters characterize the deformation of the rigid body, and in the limit of large exchange coupling should be much smaller compared to the other three. The balance equation thus becomes

$$\begin{aligned} \frac{\partial E_{ani}}{\partial \hat{\Omega}} - \frac{\partial \boldsymbol{M}}{\partial \hat{\Omega}} \cdot \boldsymbol{H} = 0, \\ \frac{\partial (E_{ex} + E_{ani})}{\partial \omega_i} - \frac{\partial \boldsymbol{M}}{\partial \omega_i} \cdot \boldsymbol{H} = 0, \end{aligned} \tag{66}$$

which are in general hard to solve, but can sometimes be simplified with additional constraints from symmetry.

## SWITCHING BETWEEN TIME-REVERSED CONFIGURATIONS

We briefly discuss here the switching process between two time-reversed states for the model system of $Mn_3Ir$. We have already shown that such a switching cannot be achieved through a single $\pi$ rotation with respect to the $(\bar{1}01)$ axis. Actually it can be realized through a single $\pi$ rotation only when the rotation axis is parallel to the ground state total magnetization. This switching path has higher barriers, however, because it causes the local moments to deviate more significantly from their local easy axes. A more probable switching process consists of three segments which rotate $\boldsymbol{M}_{\rm orb}$ from (111) to $(\bar{1}\bar{1}\bar{1})$ by going through two other equivalent (111) directions, e.g., $(111) \rightarrow (1\bar{1}1) \rightarrow (1\bar{1}\bar{1}) \rightarrow (\bar{1}\bar{1}\bar{1})$. However, in the presence of an magnetic field along $(\bar{1}\bar{1}\bar{1})$, the path will smoothly deform and for sufficiently strong fields will switch directly.

Field-induced deformation of the switching path can be seen in Figure 5, which plots the modulus of $\frac{\delta E}{\delta \boldsymbol{\omega}}$ along the same path as in Fig. 3 in the main text, but with the magnetic field along $(\bar{1}\bar{1}\bar{1})$ direction. One can see that at finite $H$ the minimum originally at $(1\bar{1}1)$ shifts to larger $\theta$.

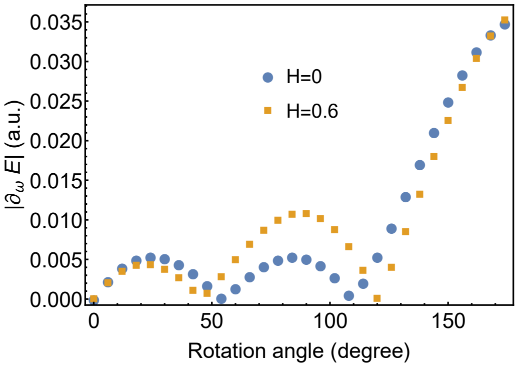


FIG. 5: Modulus of the function $\delta E/\delta \boldsymbol{\omega}$ vs. the rotation angle at zero and finite magnetic fields along $(\bar{1}\bar{1}\bar{1})$.


[1] H. Chen, Q. Niu, and A. H. MacDonald, Phys. Rev. Lett. **112**, 017205 (2014).
[2] W. Feng, G. Y. Guo, J. Zhou, Y. Yao, and Q. Niu, Phys. Rev. B **92**, 144426 (2015).
[3] G. Y. Guo, and T.-C. Wang, Phys. Rev. B **96**, 224415 (2017).
[4] J. P. Perdew, K. Burke, M. Ernzerhof, Phys. Rev. Lett. **77**, 3865 (1996).
[5] P. Giannozzi *et al.*, J. Phys.: Condens. Matter **21**, 395502 (2009).

[6] D. R. Hamann, Phys. Rev. B **88**, 085117 (2013).
[7] D. Xiao, J. Shi, and Q. Niu, Phys. Rev. Lett. **95**, 137204 (2005).
[8] X. Wang, J. R. Yates, I. Souza, and D. Vanderbilt, Phys. Rev. B **74**, 195118 (2006).
[9] M. G. Lopez, D. Vanderbilt, T. Thonhauser, and I. Souza, Phys. Rev. B **85**, 014435 (2012).
[10] N. Marzari, A. A. Mostofi, J. R. Yates, I. Souza, and D. Vanderbilt, Rev. Mod. Phys. **84**, 1419 (2012).
[11] A. A. Mostofi, J. R. Yates, Y.-S. Lee, I. Souza, D. Vanderbilt, and N. Marzari, Comput. Phys. Commun. **178**, 685 (2008).
[12] P. Bruno, *Physical origins and theoretical models of magnetic anisotropy.* Ferienkurse des Forschungszentrums Jülich, Jülich, 1993.
[13] P. K. Misra and L. Kleinman, Phys. Rev. B **72**, 4581 (1972).
[14] L. M. Roth, J. Phys. Chem. Solids **23**, 433 (1962).
[15] A. Altland and B. Simons, *Condensed Matter Field Theory*, 2nd edition.
[16] H. Fukuyama, Prog. of Theo. Phys. **45**, 704 (1971).
[17] J. Shi, G. Vignale, D. Xiao, and Q. Niu, Phys. Rev. Lett. **99**, 197202 (2007).
